# Supplementary material for: Smoothing for age-period-cohort models: a comparison between splines and random process
Source: arXiv:2312.09698 source file (2023-12-15)
Supplement: Supplementary file 1 [file supplementaryMaterial.tex]

\section{Spline basis functions}

Using a toy dataset defined by $A = 15$ ages and five knots, Figure \ref{Fig: differentBasisExamples} shows the examples the sets of bases defined by a cubic regression spline (CRS), B-spline (BS) and thin plate regression spline (TPRS). The bases are not orthogonalised to either an intercept or linear slope. 

\begin{figure}[!h]
    \centering
    \includegraphics[width=\linewidth]{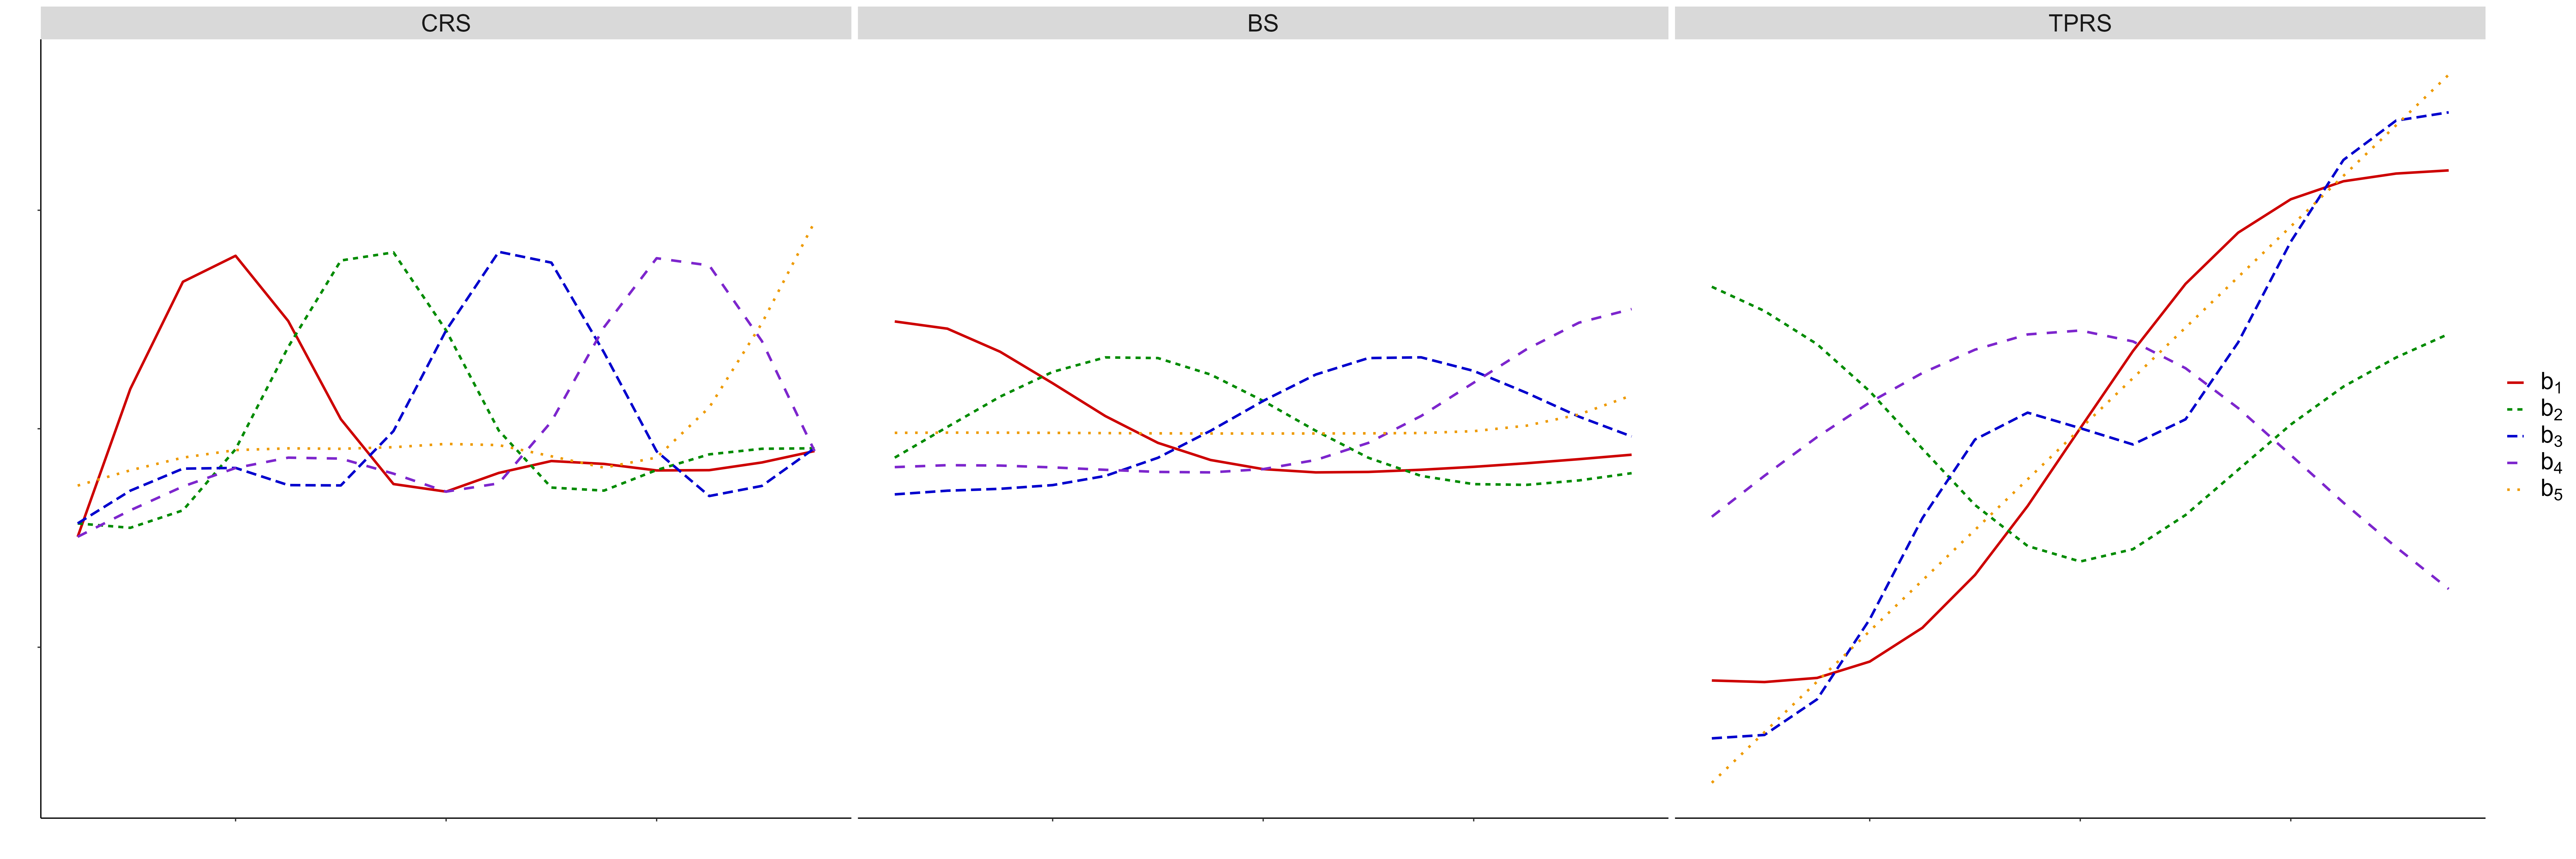}
    \caption{Examples of the basis functions for a cubic regression spline, B-spline and thin plate regression spline.}
    \label{Fig: differentBasisExamples}
\end{figure}

\clearpage

\section{Model scores from simulation study}

Table \ref{Tab: Simulation study model fit scores} shows the mean values for the model fit scores. These values correspond to the thick line within the `box' part of the box plots in the main manuscript. 

\begin{table}[!h]
    \centering
    \caption{Model scores for the simulation study. 
    %The first two columns define the model type and specifications. The next four columns are the model score, the Mean Absolute Error, Mean Square Error, Interval Score and (uncertainty) width. The top six columns are the results for estimation and the bottom six are for prediction.
    }
    \label{Tab: Simulation study model fit scores}
    \resizebox{\textwidth}{!}{%
    \begin{tabular}{cc|cccc}
        \hline
        \multicolumn{6}{c}{\textbf{Estimation} $\pa{\times 10^{-2}}$} \\
        \textbf{Model Type} & \textbf{Model Specification} & \textbf{Mean Absolute Error} & \textbf{Mean Square Error} & \textbf{Interval Score} & \textbf{Width} \\
        \hline
        \multirow{3}{*}{\textbf{Penalised Spline}} & CRS & 13.6459 & 3.0136 & 368.7563 & 10.8174 \\
         & BS & 13.6484 & 3.0144 & 369.5985 & 10.7644 \\
         & TPRS & 13.6511 & 3.0154 & 369.0794 & 10.8027 \\
        \hline
        \multirow{3}{*}{\textbf{Random Walk 2}} & U = 1 & 13.4897 & 2.9475 & 317.1453 & 14.2242 \\
         & U = 3 & 13.4848 & 2.9453 & 315.9283 & 14.3054 \\
         & U = 6 & 13.4833 & 2.9447 & 315.6193 & 14.3261 \\
        \hline
        \multicolumn{6}{c}{\textbf{Prediction} $\pa{\times 10^{-2}}$} \\
        \textbf{Model Type} & \textbf{Model Specification} & \textbf{Mean Absolute Error} & \textbf{Mean Square Error} & \textbf{Interval Score} & \textbf{Width} \\
        \hline
        \multirow{3}{*}{\textbf{Penalised Spline}} & CRS & 14.0717 & 3.1161 & 317.8736 & 16.0993 \\
         & BS & 14.0775 & 3.1187 & 316.8082 & 16.3022 \\
         & TPRS & 14.0690 & 3.1102 & 318.6231 & 15.9625 \\
        \hline
        \multirow{3}{*}{\textbf{Random Walk 2}} & U = 1 & 14.0885 & 3.1487 & 190.1655 & 32.0939 \\
         & U = 3 & 14.0915 & 3.1509 & 188.1159 & 32.5784 \\
         & U = 6 & 14.0930 & 3.1518 & 187.6254 & 32.6871 \\
        \hline
    \end{tabular}%
    }
\end{table}

\clearpage

\section{Heatmaps for complete data for mental health outcomes}

Figure \ref{Fig: ObservedHeatmap} shows heatmaps of deaths due to alcohol and self harm for the years 2006 -- 2021 and ages 10 -- 84. In the main analysis, we considered only the ages 25 -- 84 as there was a large difference between the ages 10 -- 24 and 25 -- 84. This is more notable for the self harm related deaths. 

\begin{figure}[!h]
    \centering
    \begin{subfigure}{.5\textwidth}
        \centering
        \includegraphics[width=\linewidth]{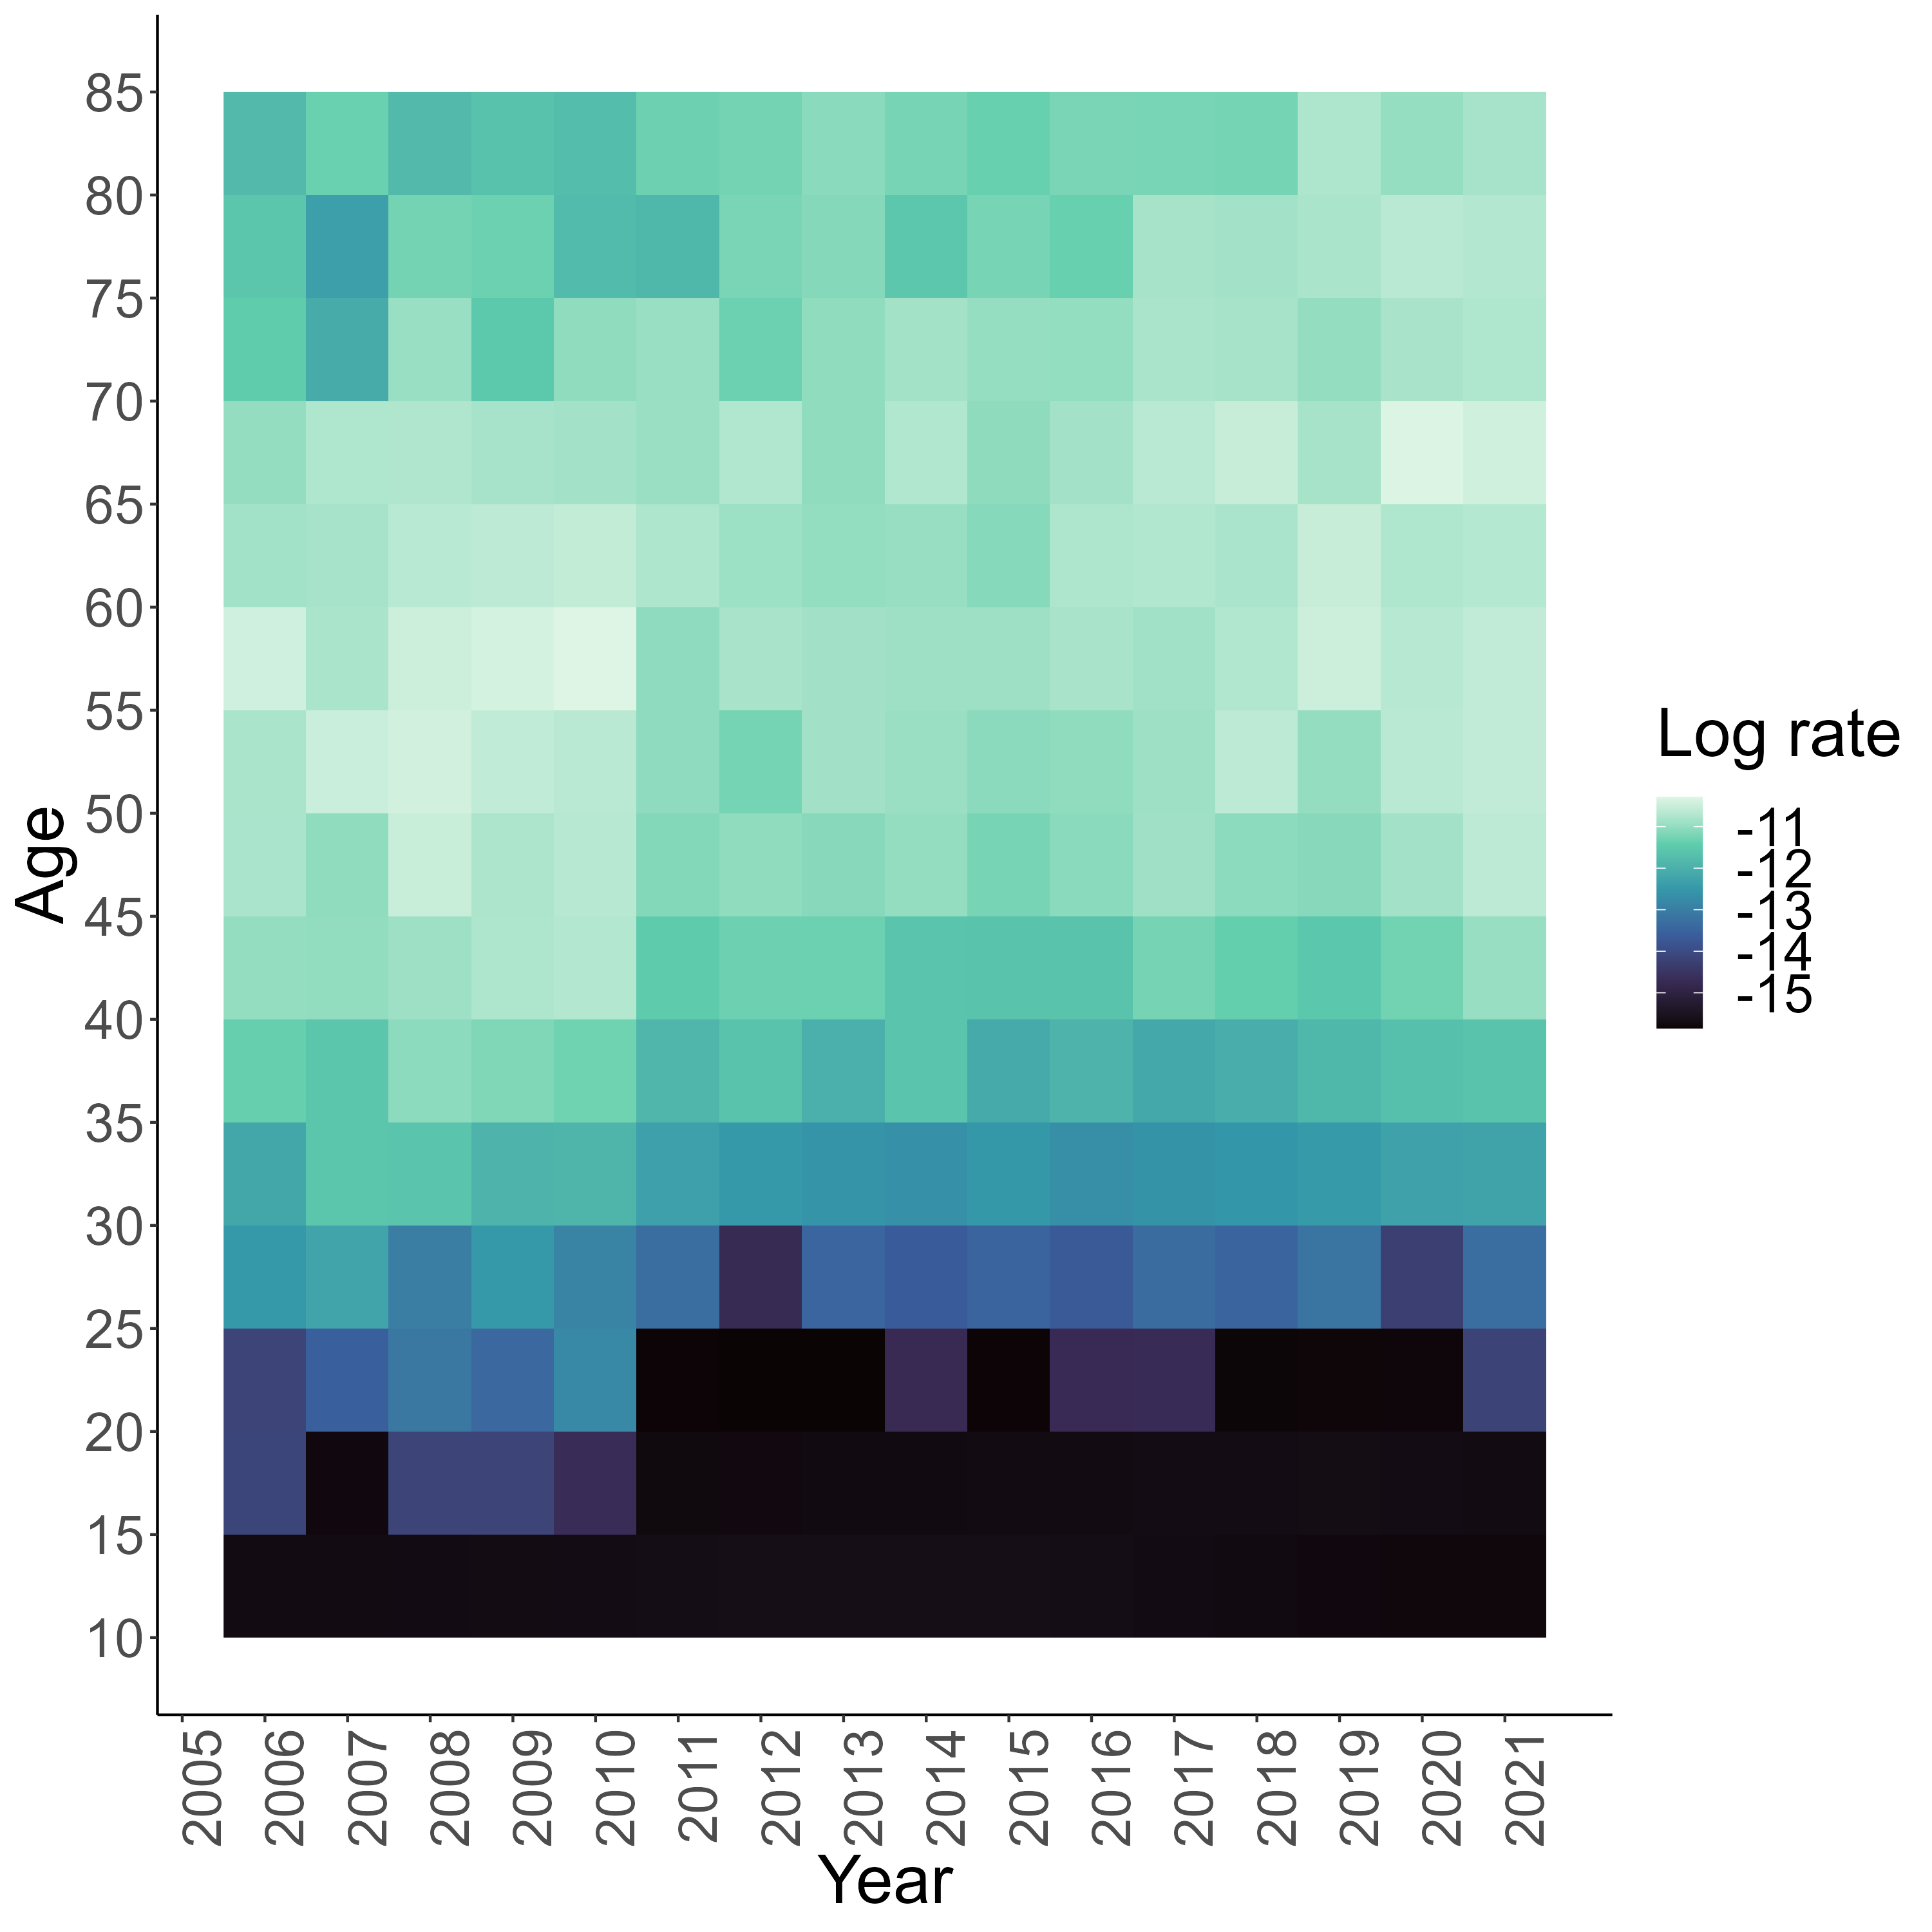}
        \caption{Alcohol related deaths}
        \label{Fig: alcoholObservedHeatmap}
    \end{subfigure}%
    \begin{subfigure}{.5\textwidth}
        \centering
        \includegraphics[width=\linewidth]{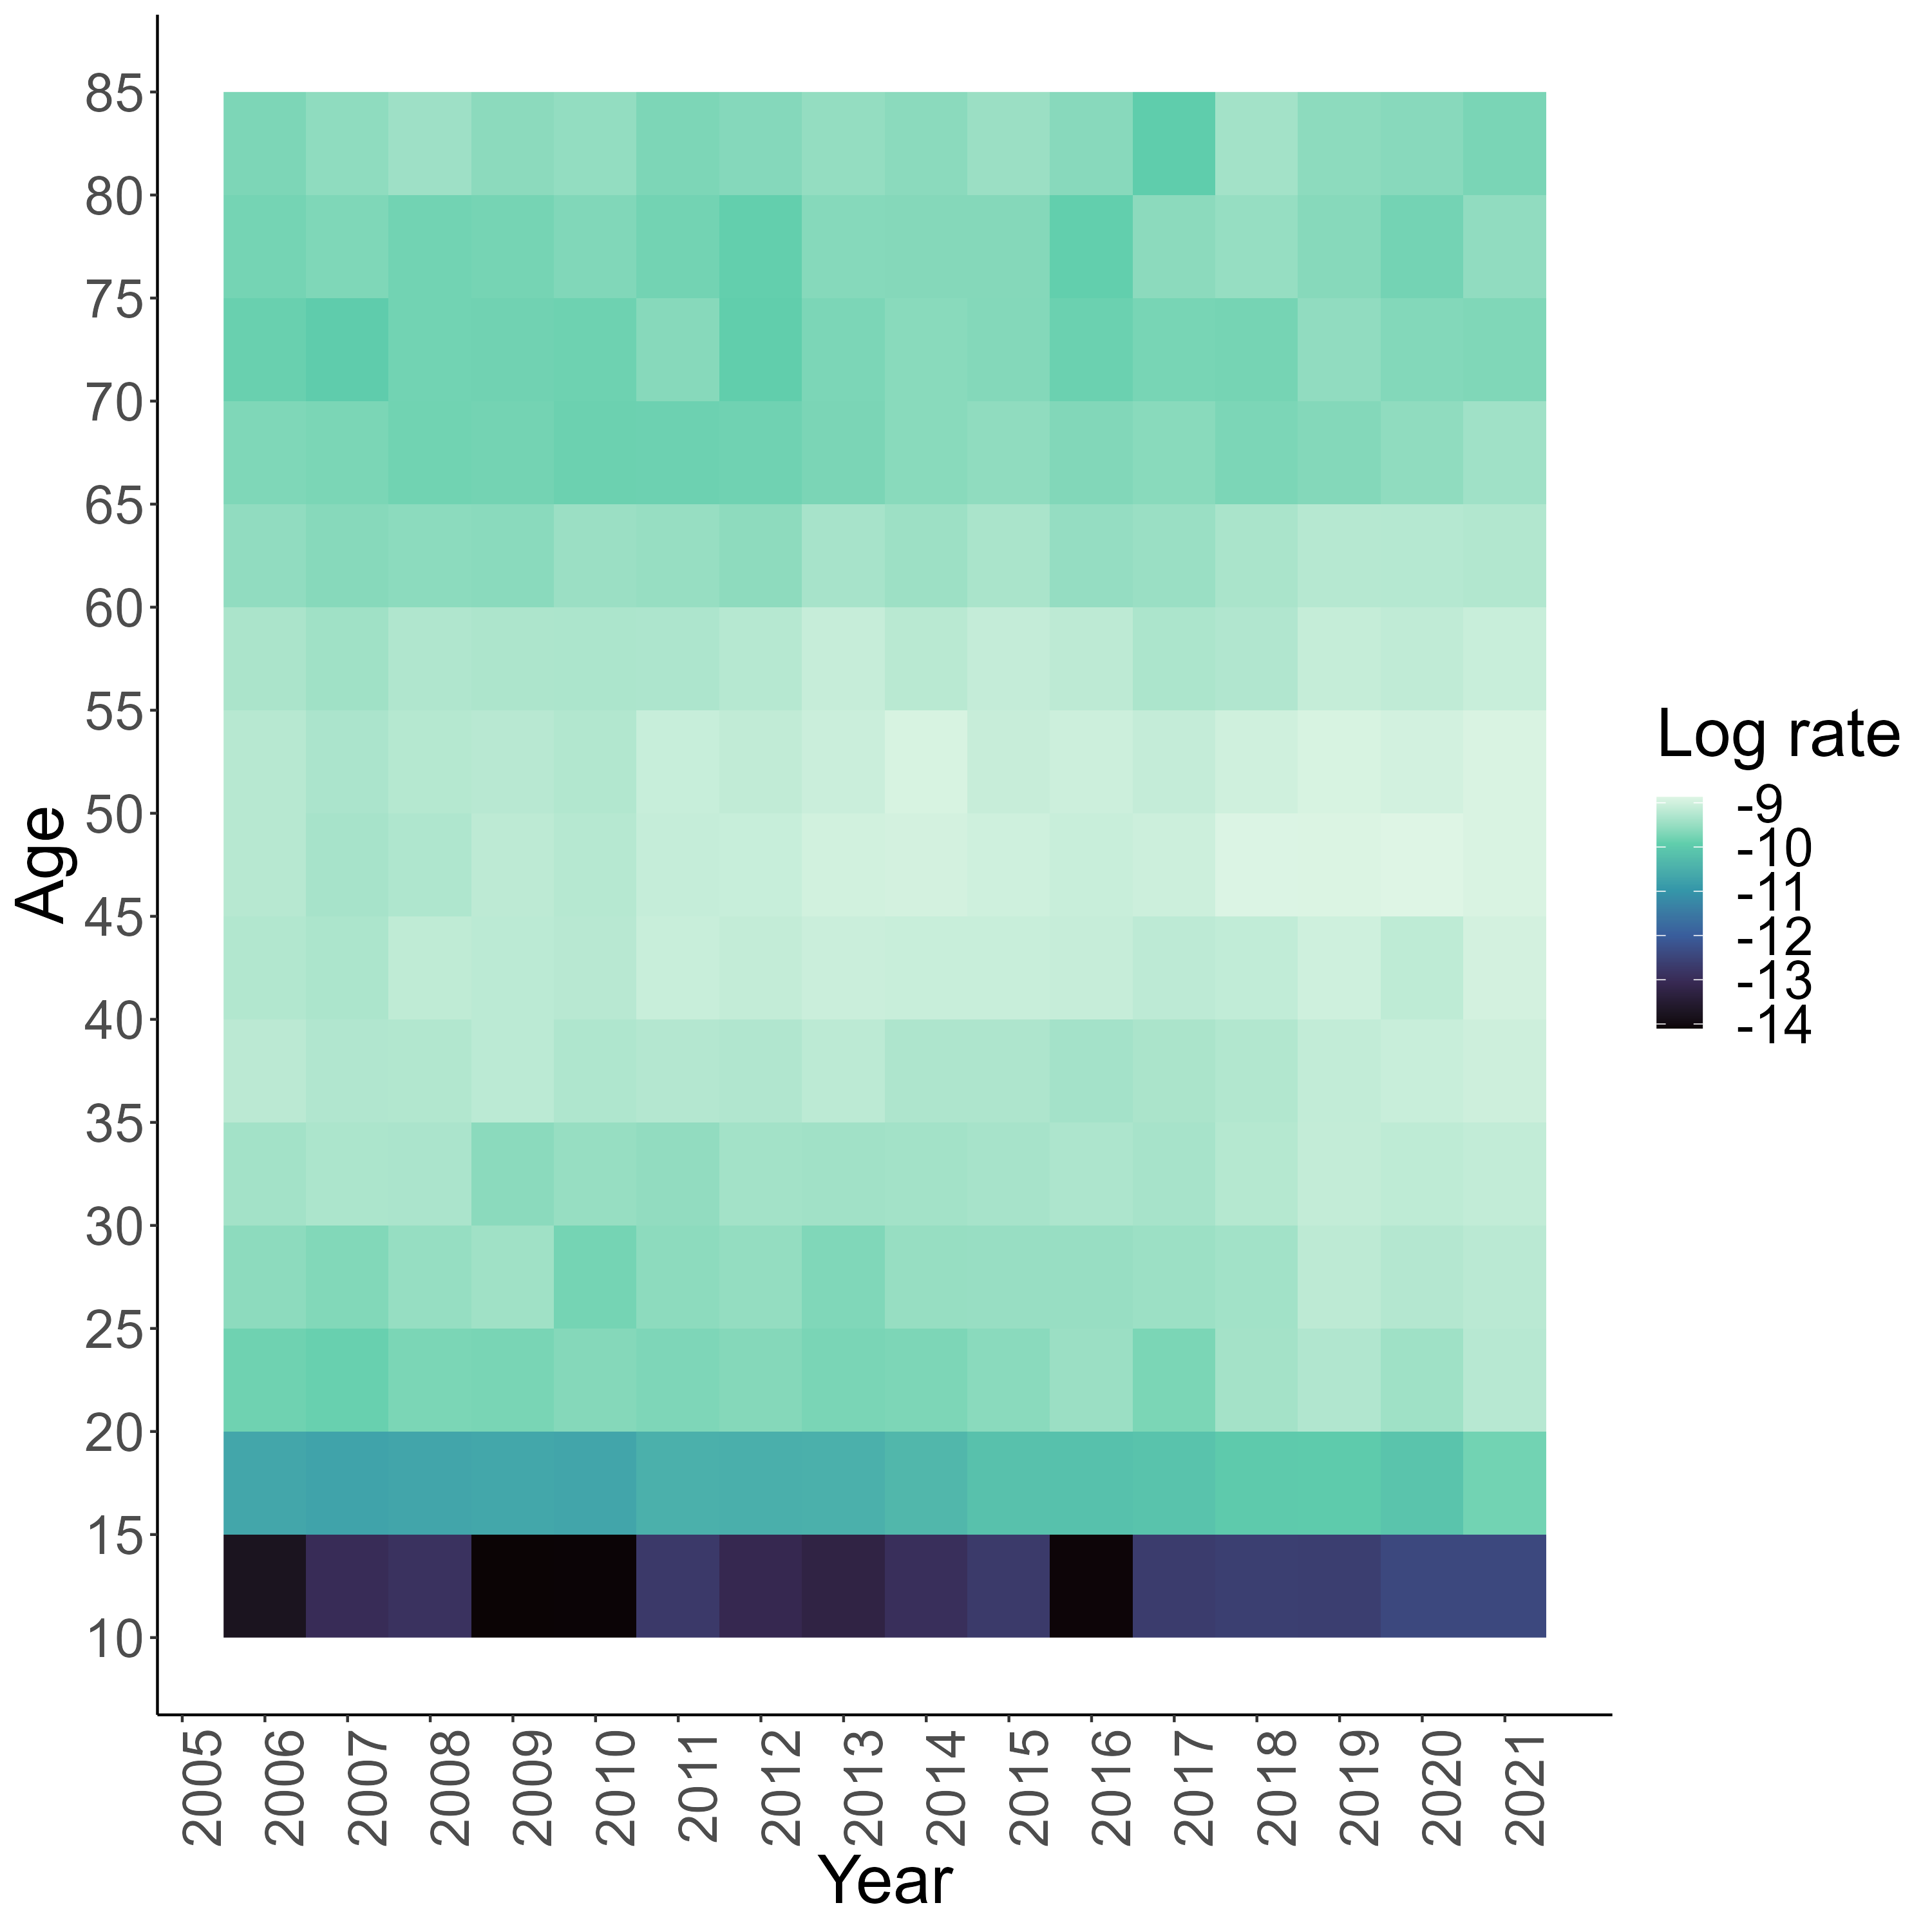}
        \caption{Self harm related deaths}
        \label{Fig: selfHarmObservedHeatmap}
    \end{subfigure}
    \caption{Deaths due to alcohol and self harm for the years 2006 -- 2021 and ages 10 -- 84. Period is grouped into single years and operates along the $x$-axis. Age is grouped into five-year ages groups and operates along the $y-axis$. Cohort operates along the $y = x$ axis. Suicides are reported as log-rates with the dark-to-light colouring indicating lower-to-higher suicide rates.}
    \label{Fig: ObservedHeatmap}
\end{figure}

\clearpage

\section{Heatmaps from model fits of alcohol related deaths}

Figure \ref{Fig: alcoholPredictedHeatmap} shows the estimated and predicted values from the penalised spline and RW2 models for alcohol related deaths. The dashed red line indicates where the estimation ends and prediction starts.

\begin{figure}[!h]
    \centering
    \begin{subfigure}{.5\textwidth}
        \centering
        \includegraphics[width=\linewidth]{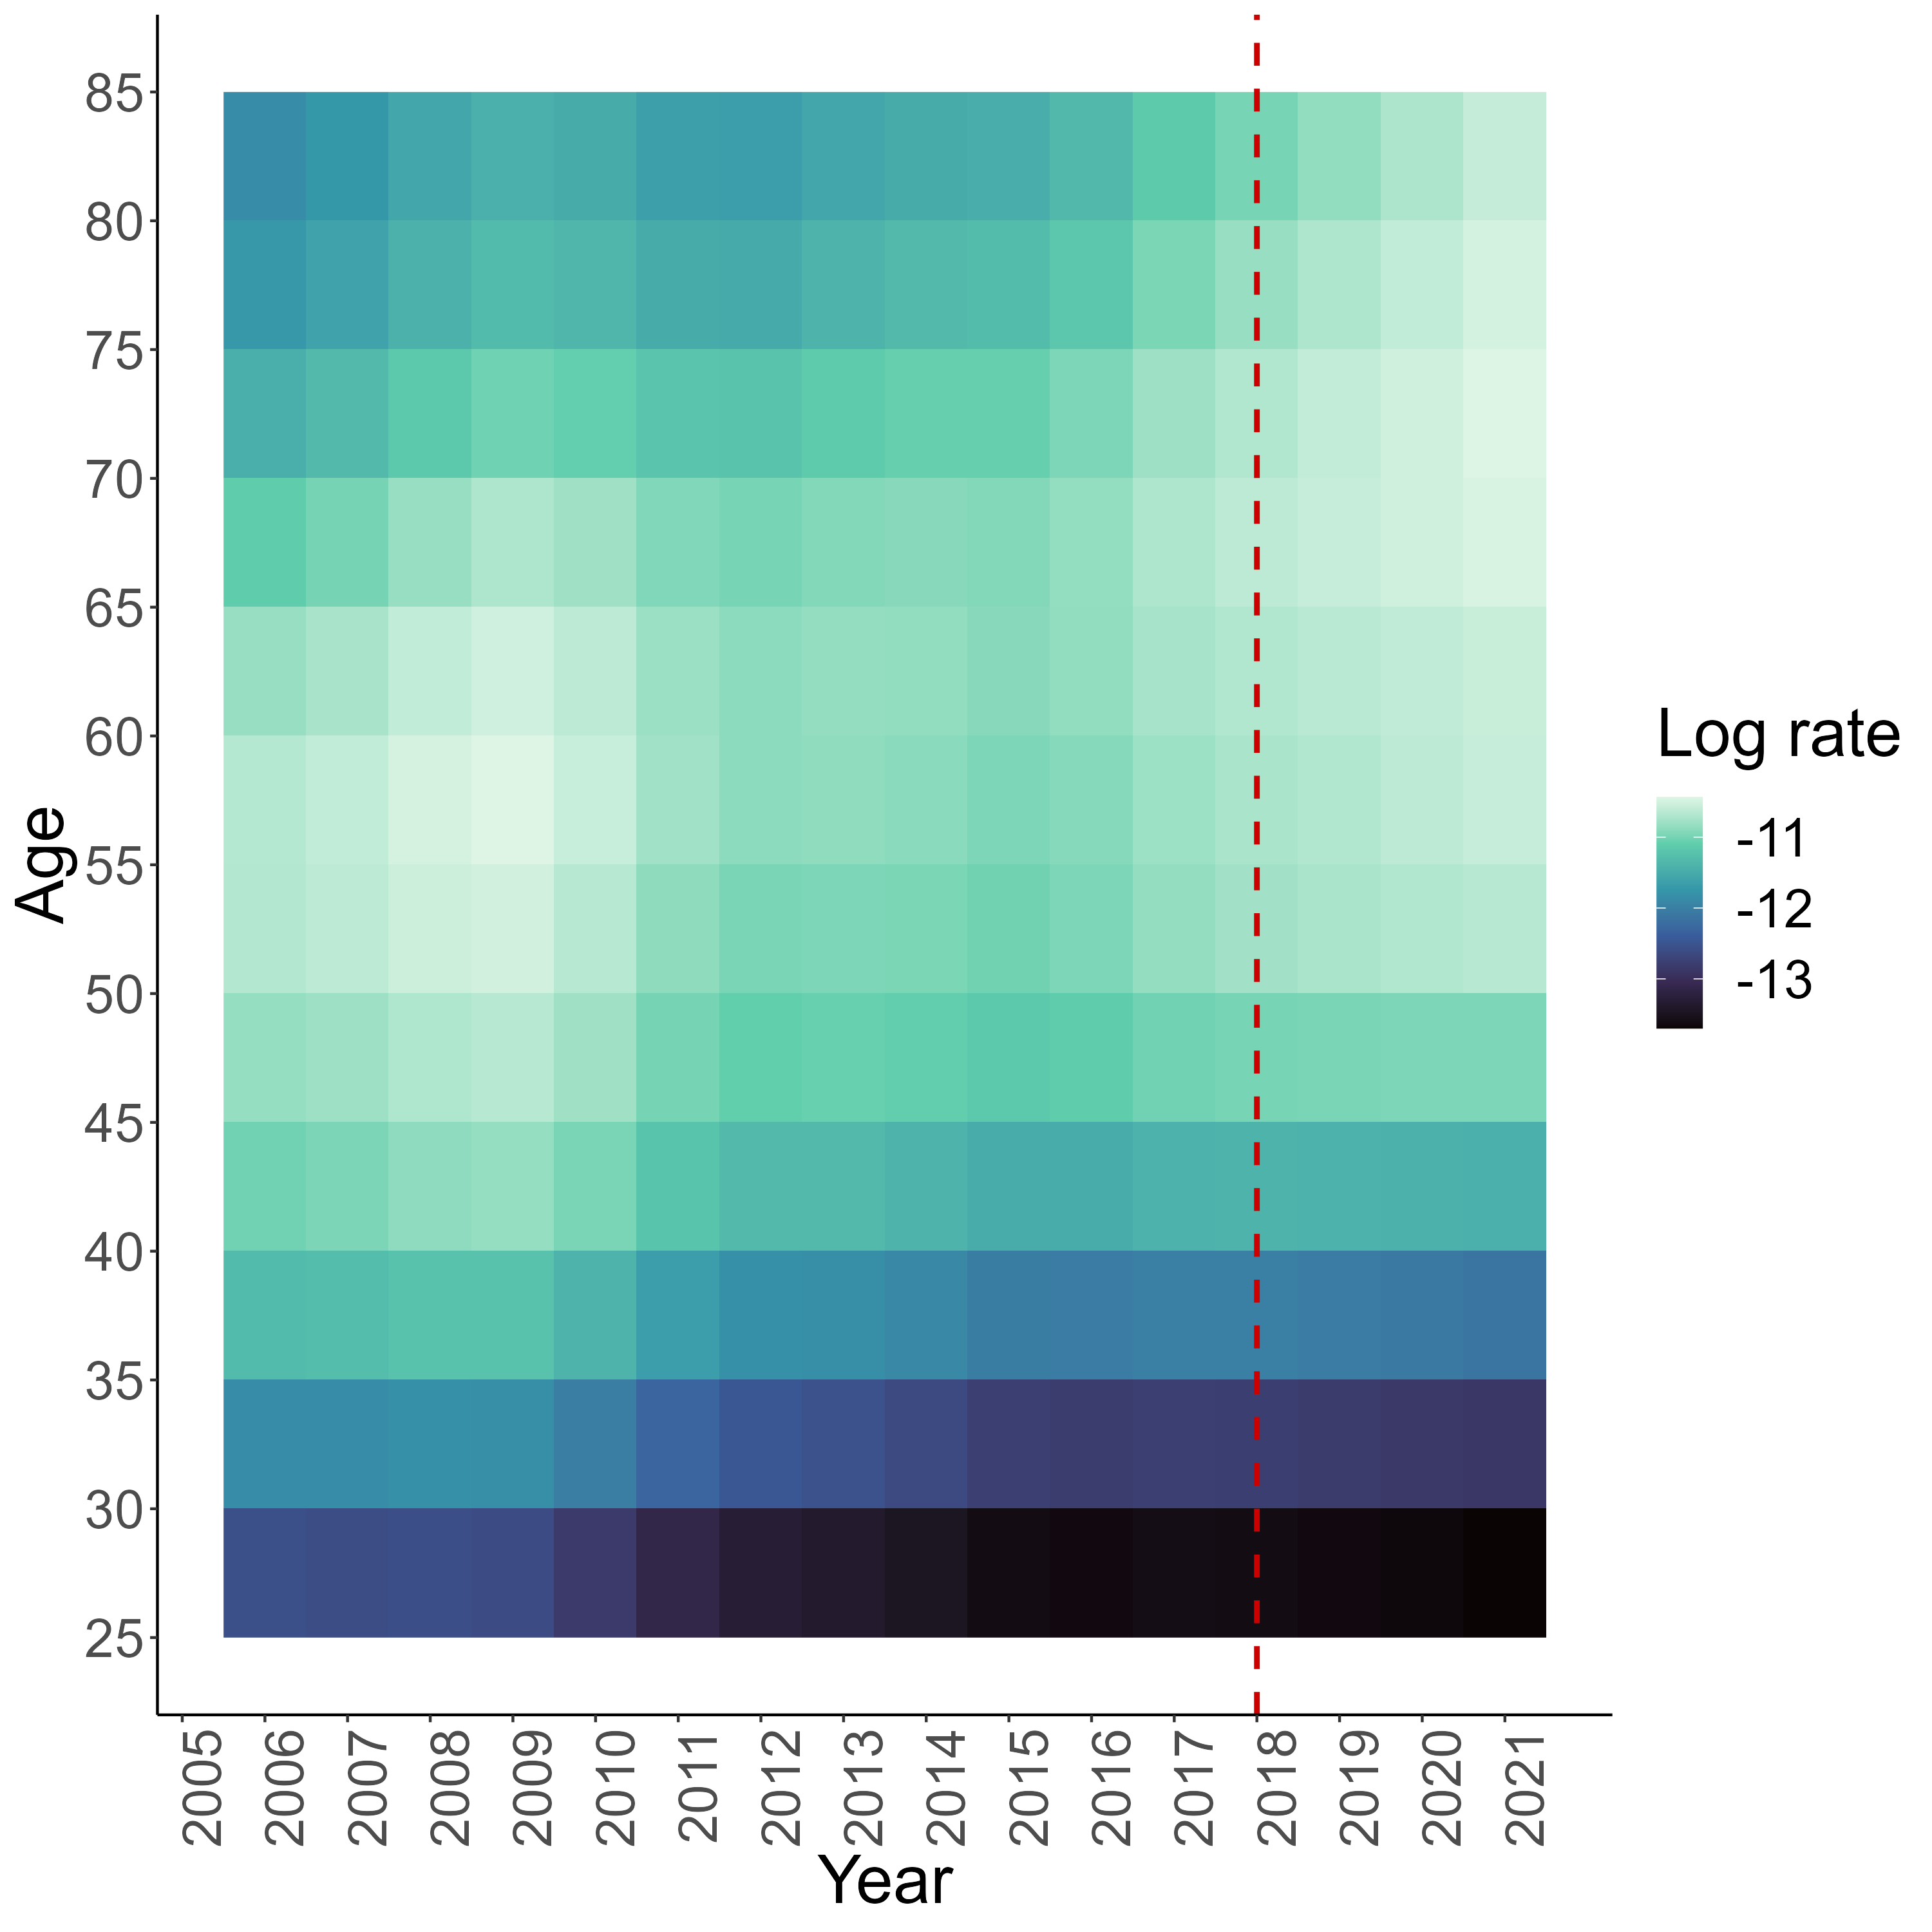}
        \caption{Spline predictions}
        \label{Fig: alcoholPredictedHeatmap_spline}
    \end{subfigure}%
    \begin{subfigure}{.5\textwidth}
        \centering
        \includegraphics[width=\linewidth]{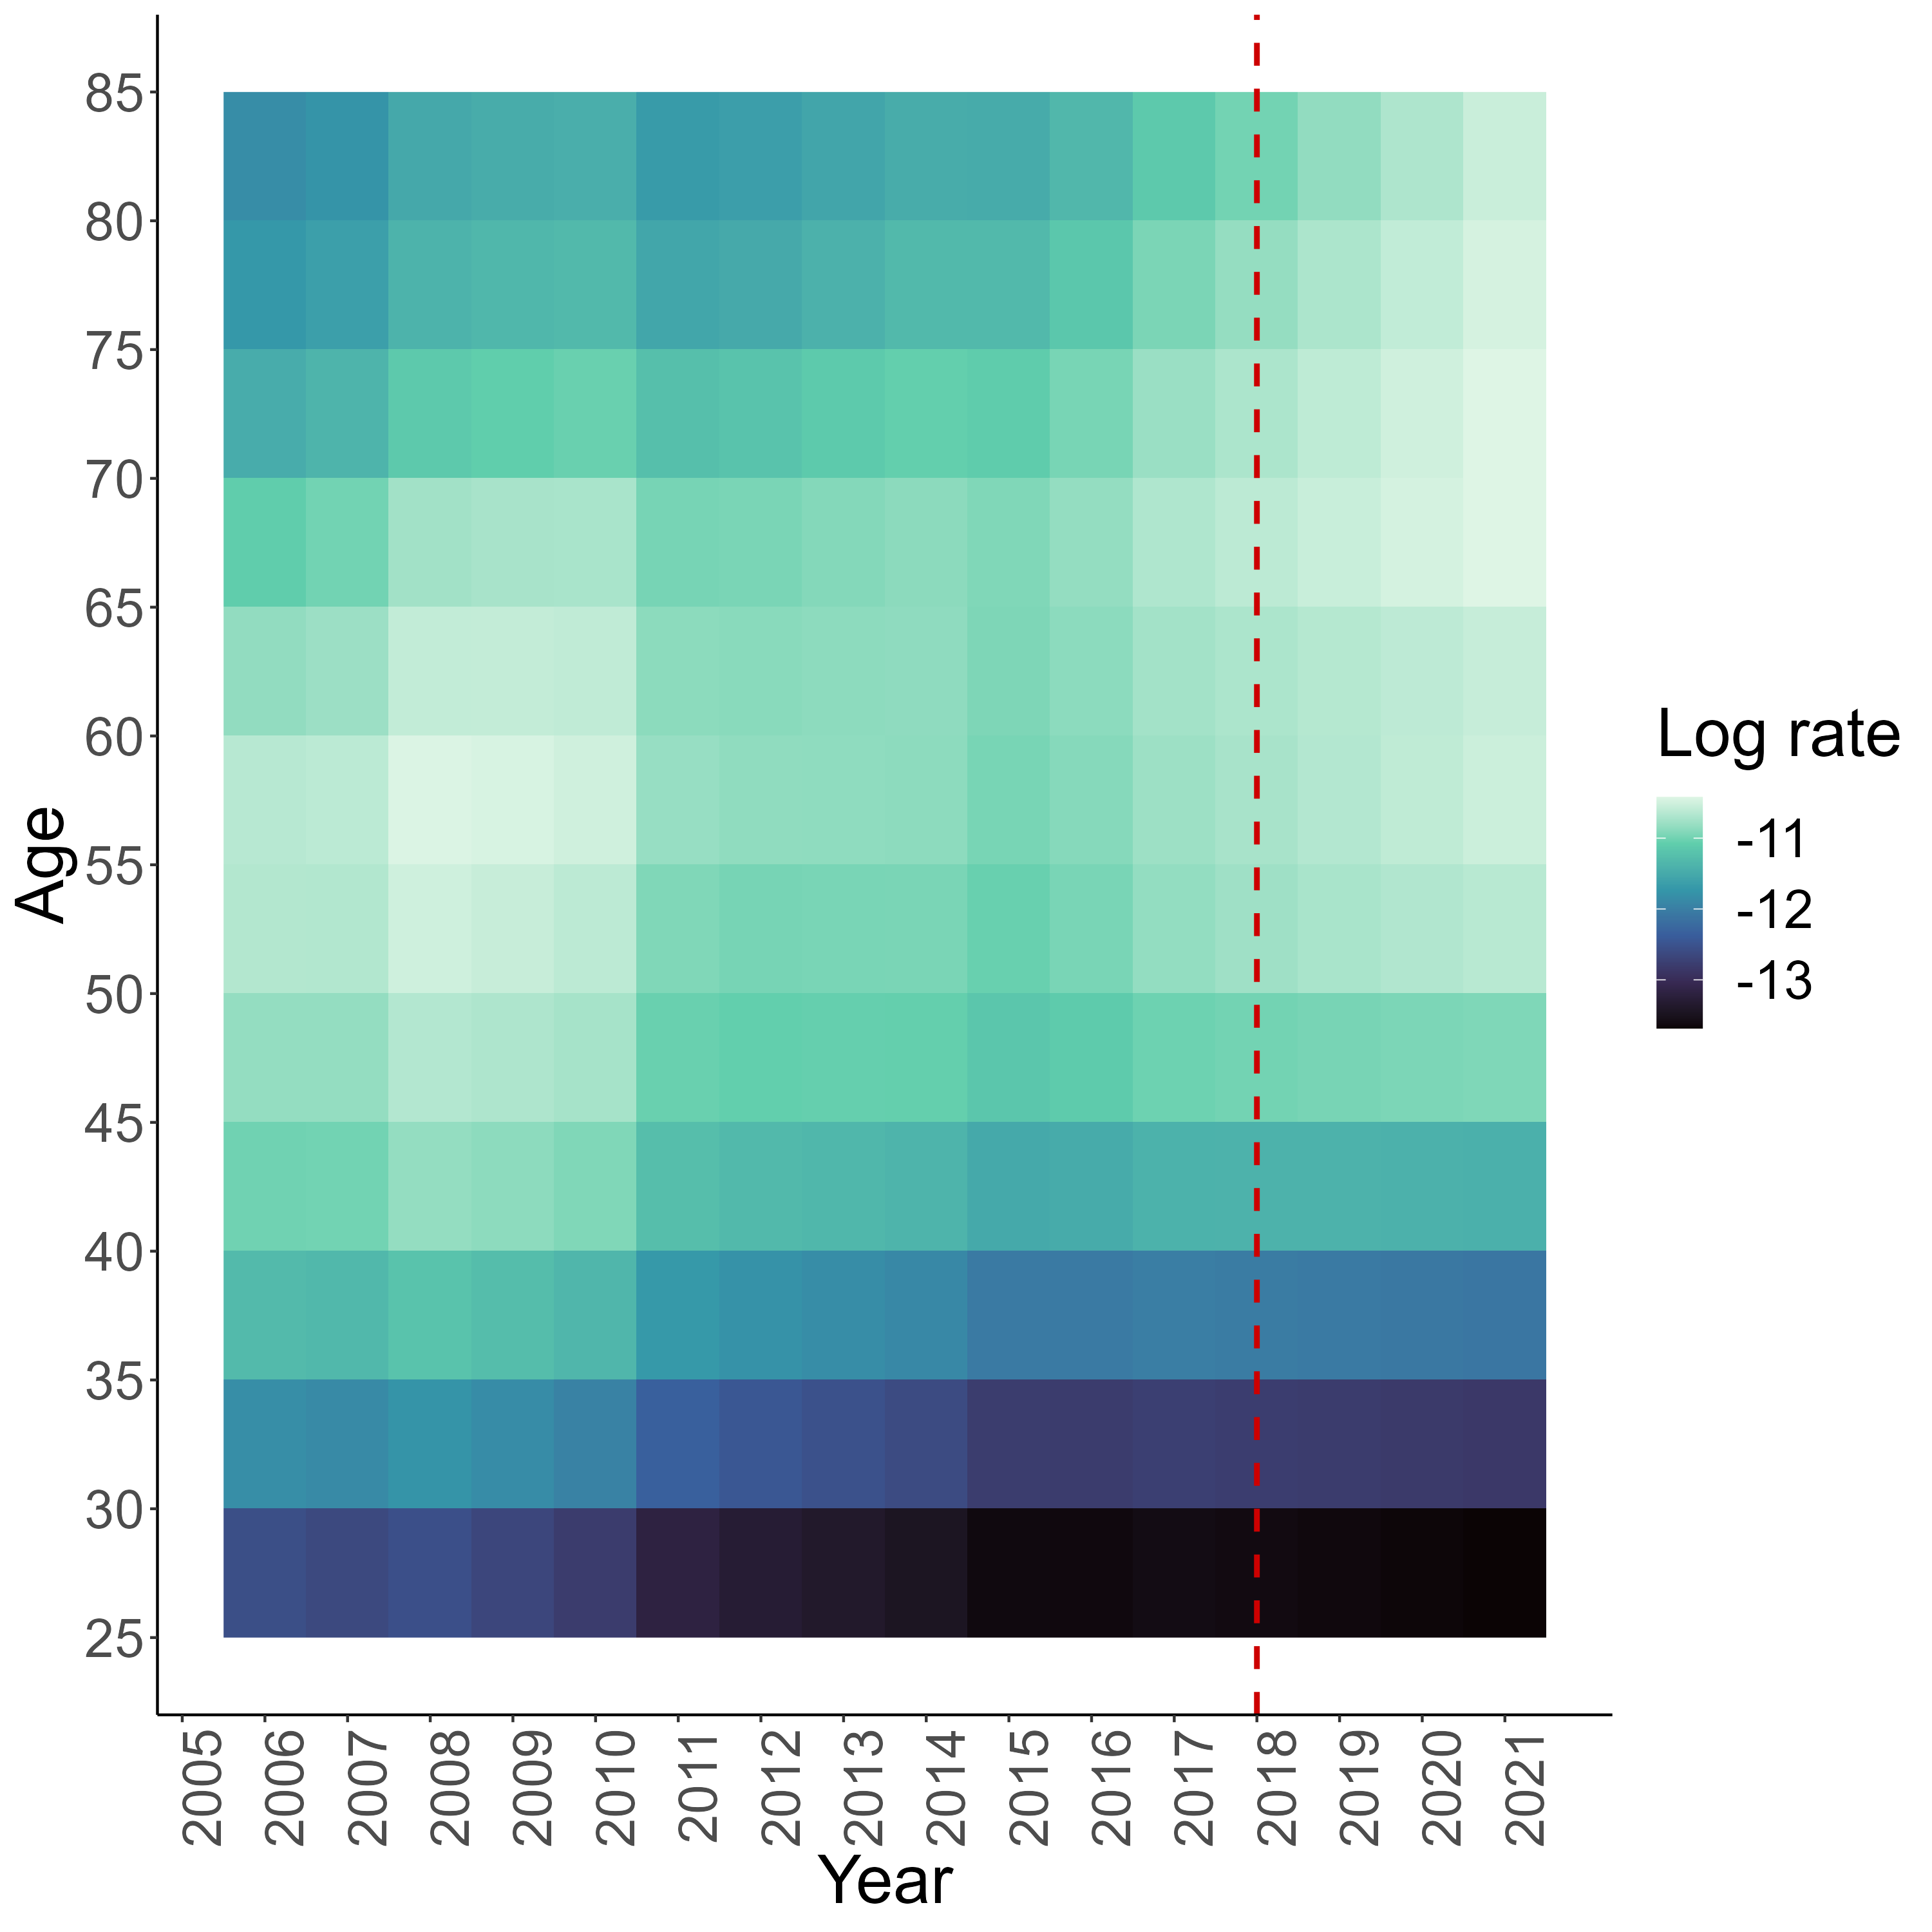}
        \caption{Random walk 2 predictions}
        \label{Fig: alcoholPredictedHeatmap_rw2}
    \end{subfigure}
    \caption{Estimates and predictions of deaths due to alcohol for the years 2006 -- 2021 and ages 25 -- 84. The left hand plot (a) is from the spline model and the right hand plot (b) is from the random walk 2 model.}
    \label{Fig: alcoholPredictedHeatmap}
\end{figure}

\clearpage

\section{Heatmaps from model fits of self harm related deaths}

Figure \ref{Fig: selfHarmPredictedHeatmap} shows the estimated and predicted values from the penalised spline and RW2 models for self-harm related deaths. The dashed red line indicates where the estimation ends and prediction starts.

\begin{figure}[!h]
    \centering
    \begin{subfigure}{.5\textwidth}
        \centering
        \includegraphics[width=\linewidth]{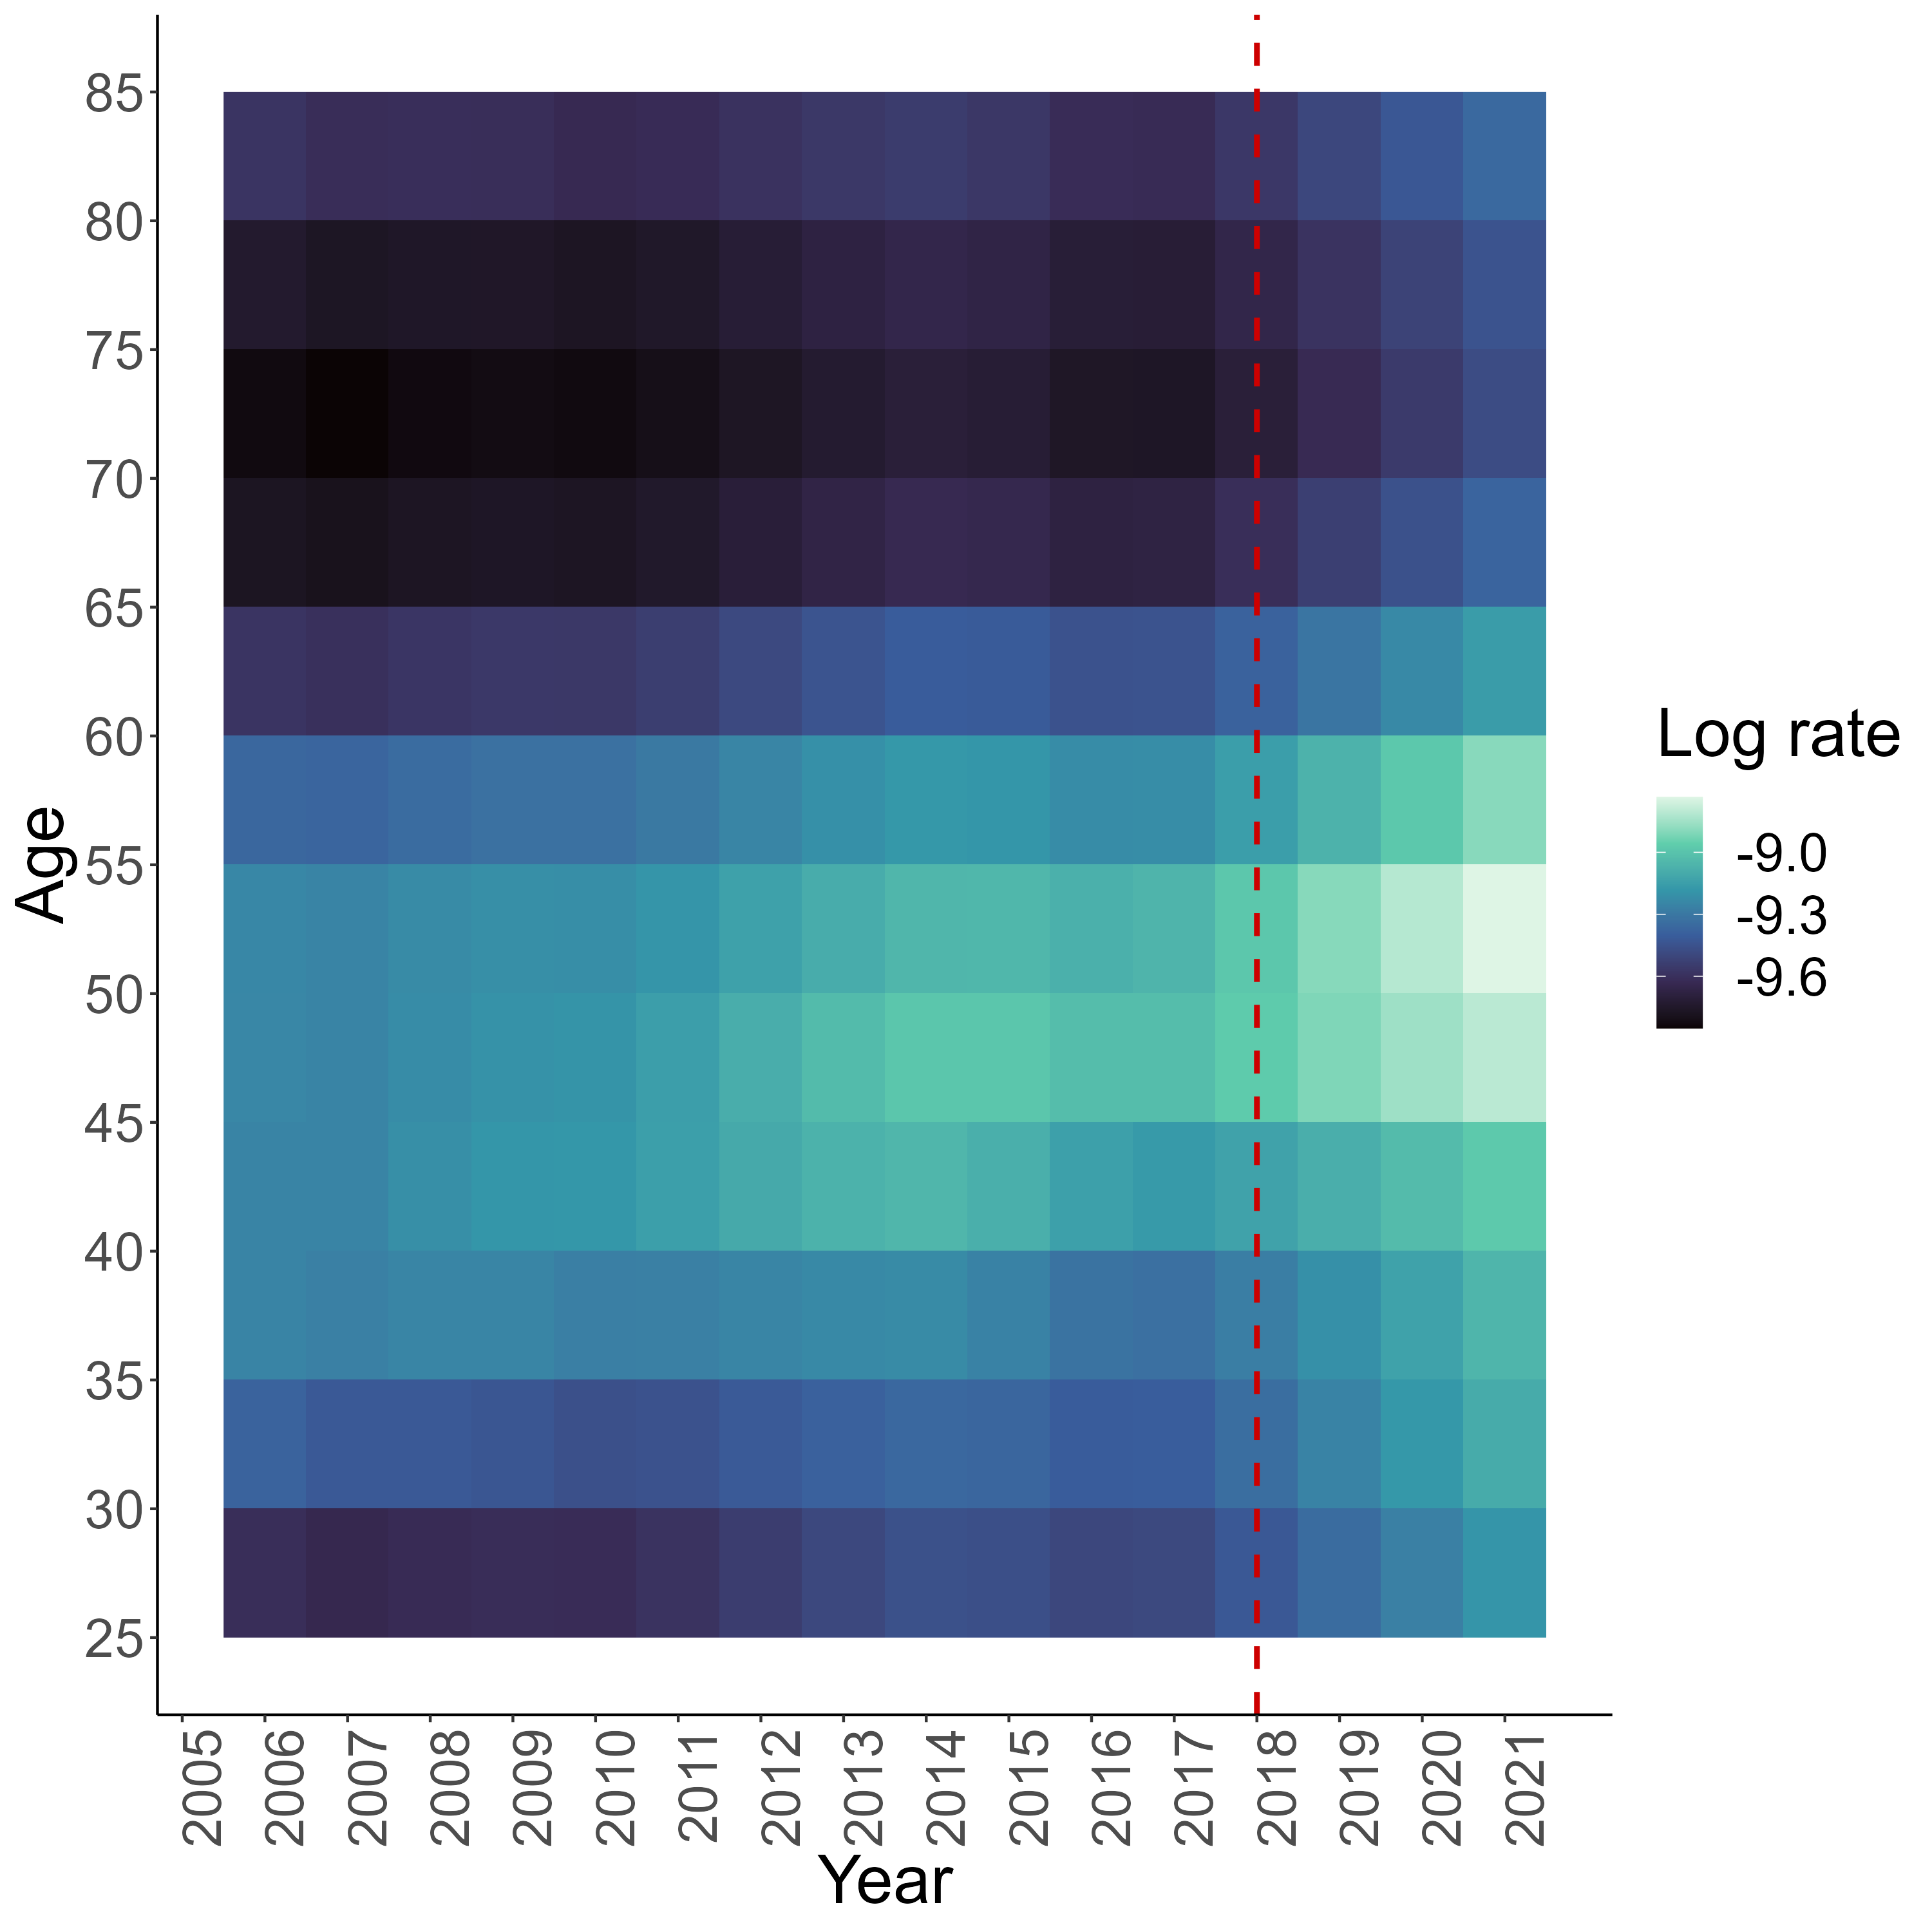}
        \caption{Spline predictions}
        \label{Fig: selfHarmPredictedHeatmap_spline}
    \end{subfigure}%
    \begin{subfigure}{.5\textwidth}
        \centering
        \includegraphics[width=\linewidth]{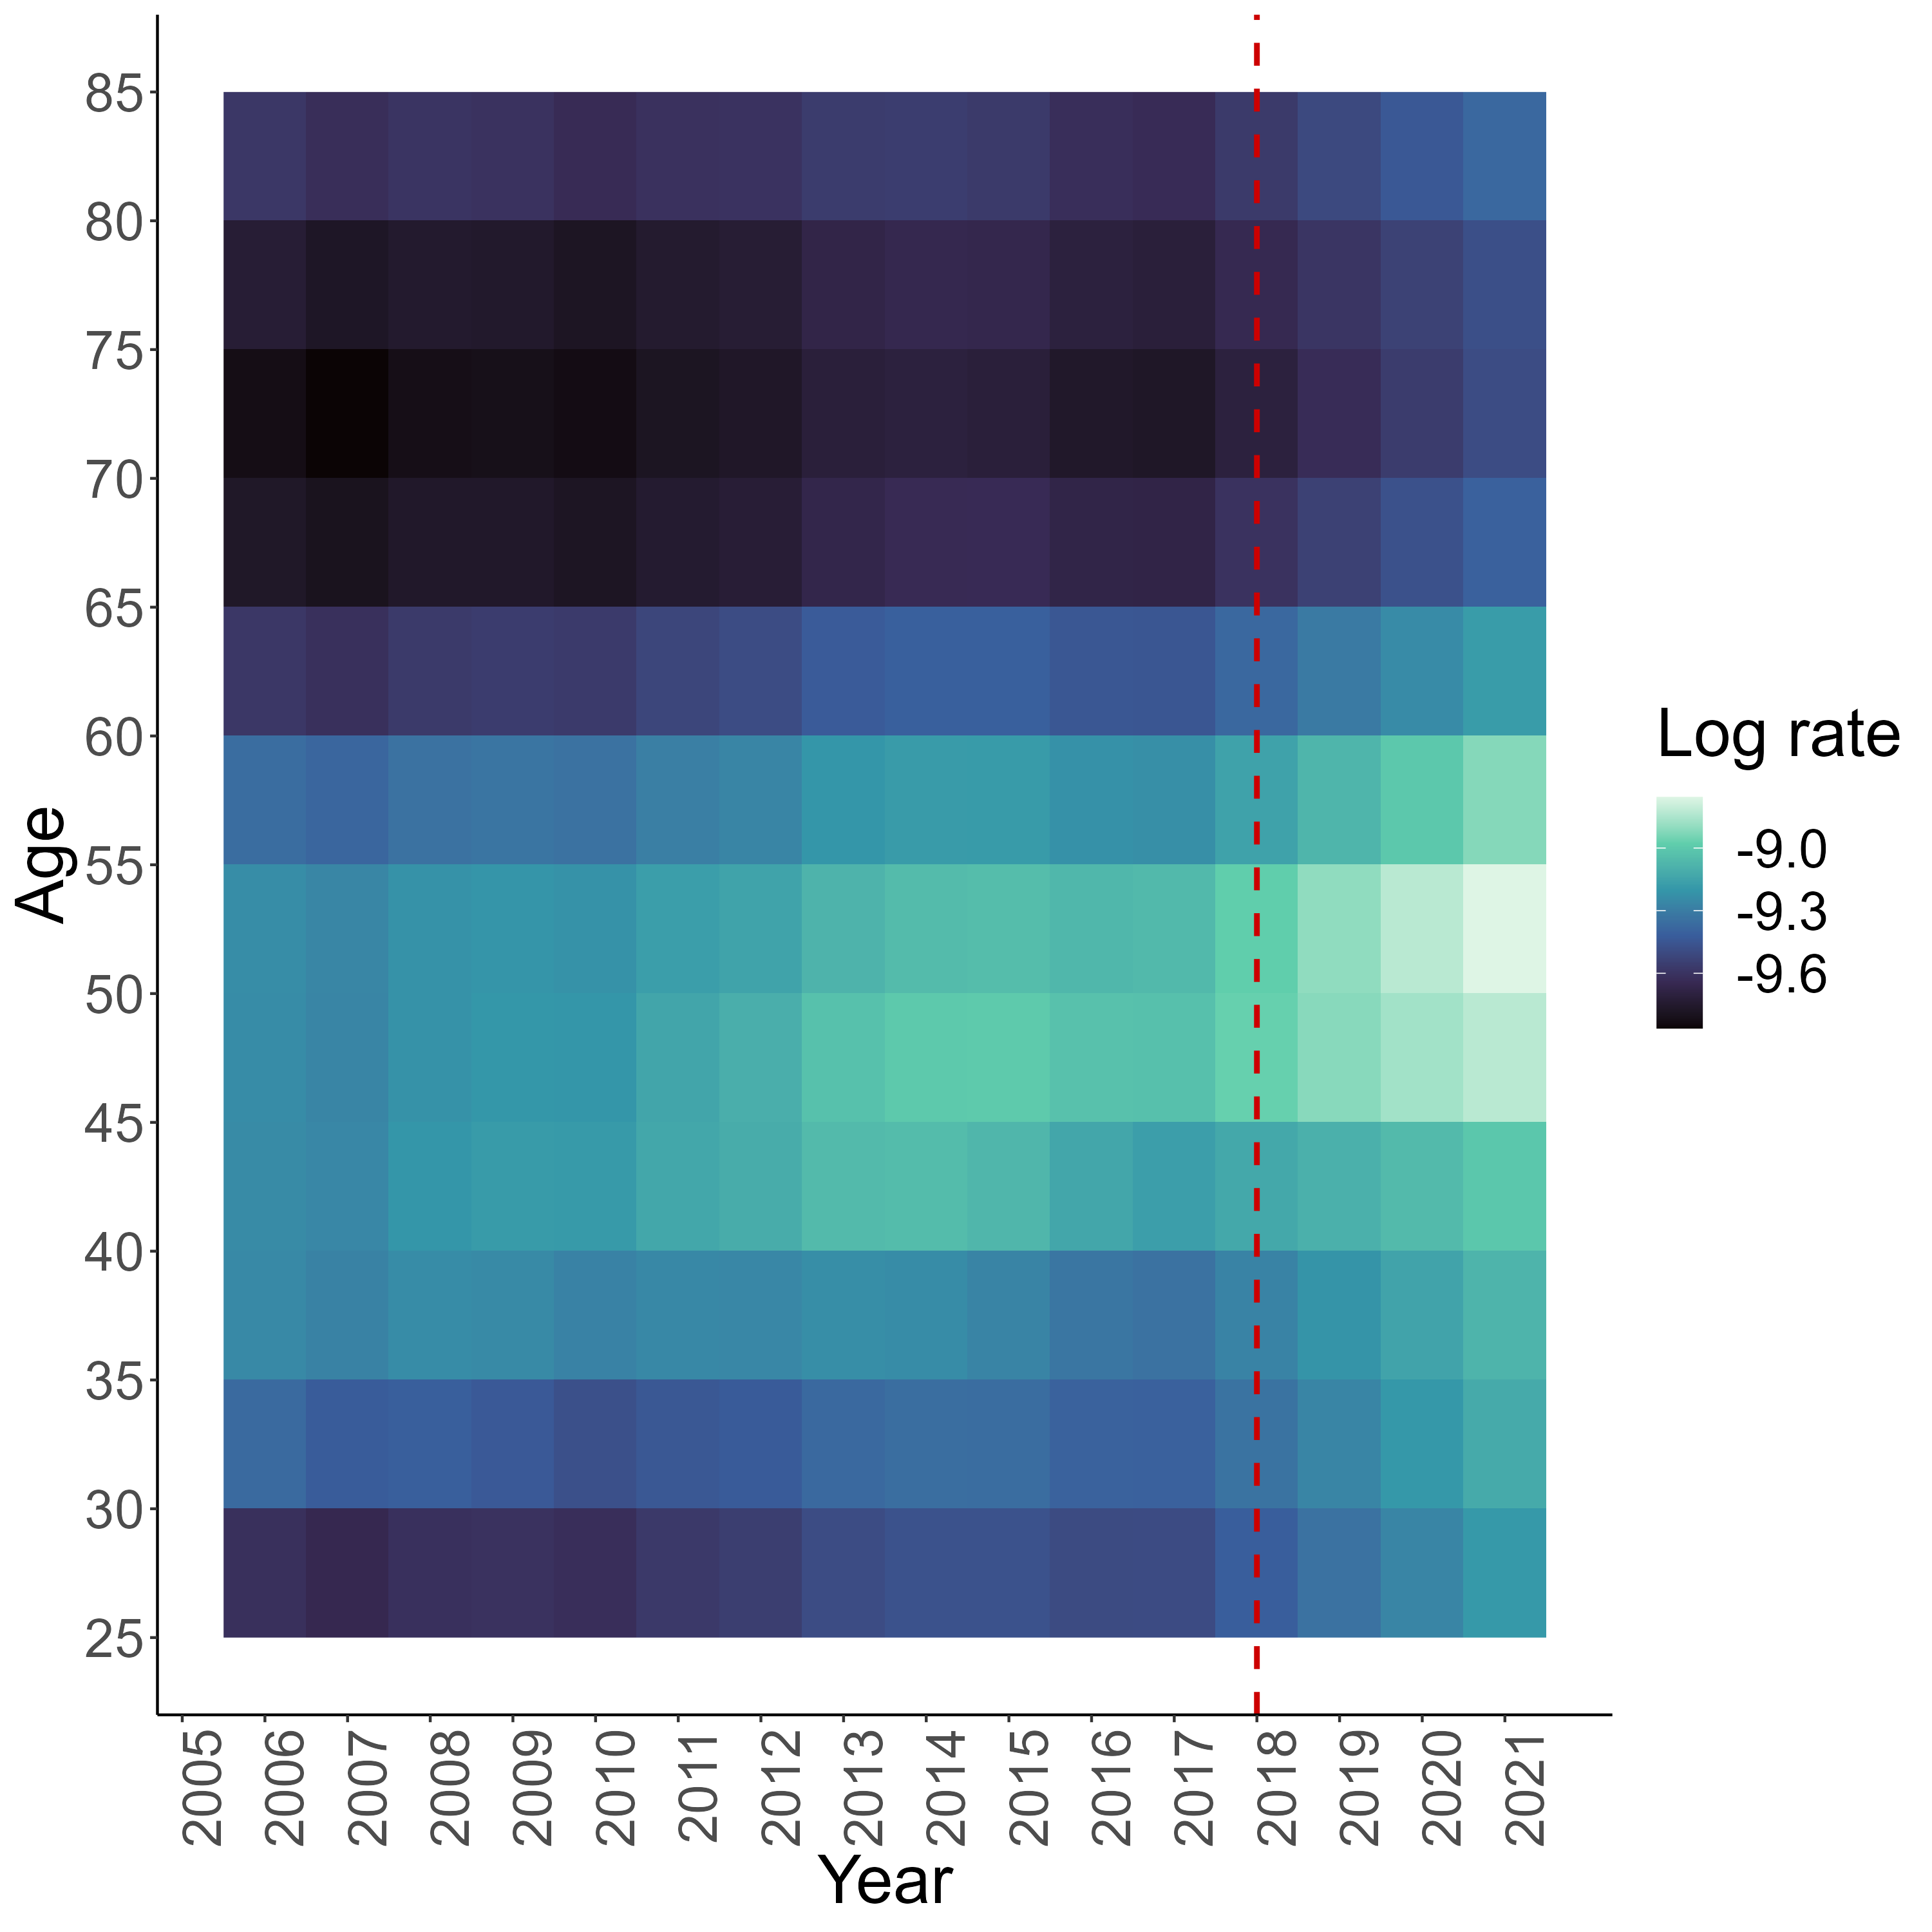}
        \caption{Random walk 2 predictions}
        \label{Fig: selfHarmPredictedHeatmap_rw2}
    \end{subfigure}
    \caption{Estimates and predictions of deaths due to self harm for the years 2006 -- 2021 and ages 25 -- 84. The left hand plot (a) is from the spline model and the right hand plot (b) is from the random walk 2 model.}
    \label{Fig: selfHarmPredictedHeatmap}
\end{figure}

\clearpage

\section{Spline and Random Walk Comparison Plots}

Figure \ref{Fig: Predicted_splineVsRW2} shows the estimated and predicted fitted values for the spline and RW2 models for both the alcohol and self harm related deaths. In each scenario, both sets of estimated and predicted values fall along the $y = x$ axis, hence are similar to one another.

\begin{figure}[!h]
    \centering
    \begin{subfigure}{.49\textwidth}
        \centering
        \includegraphics[width=\linewidth]{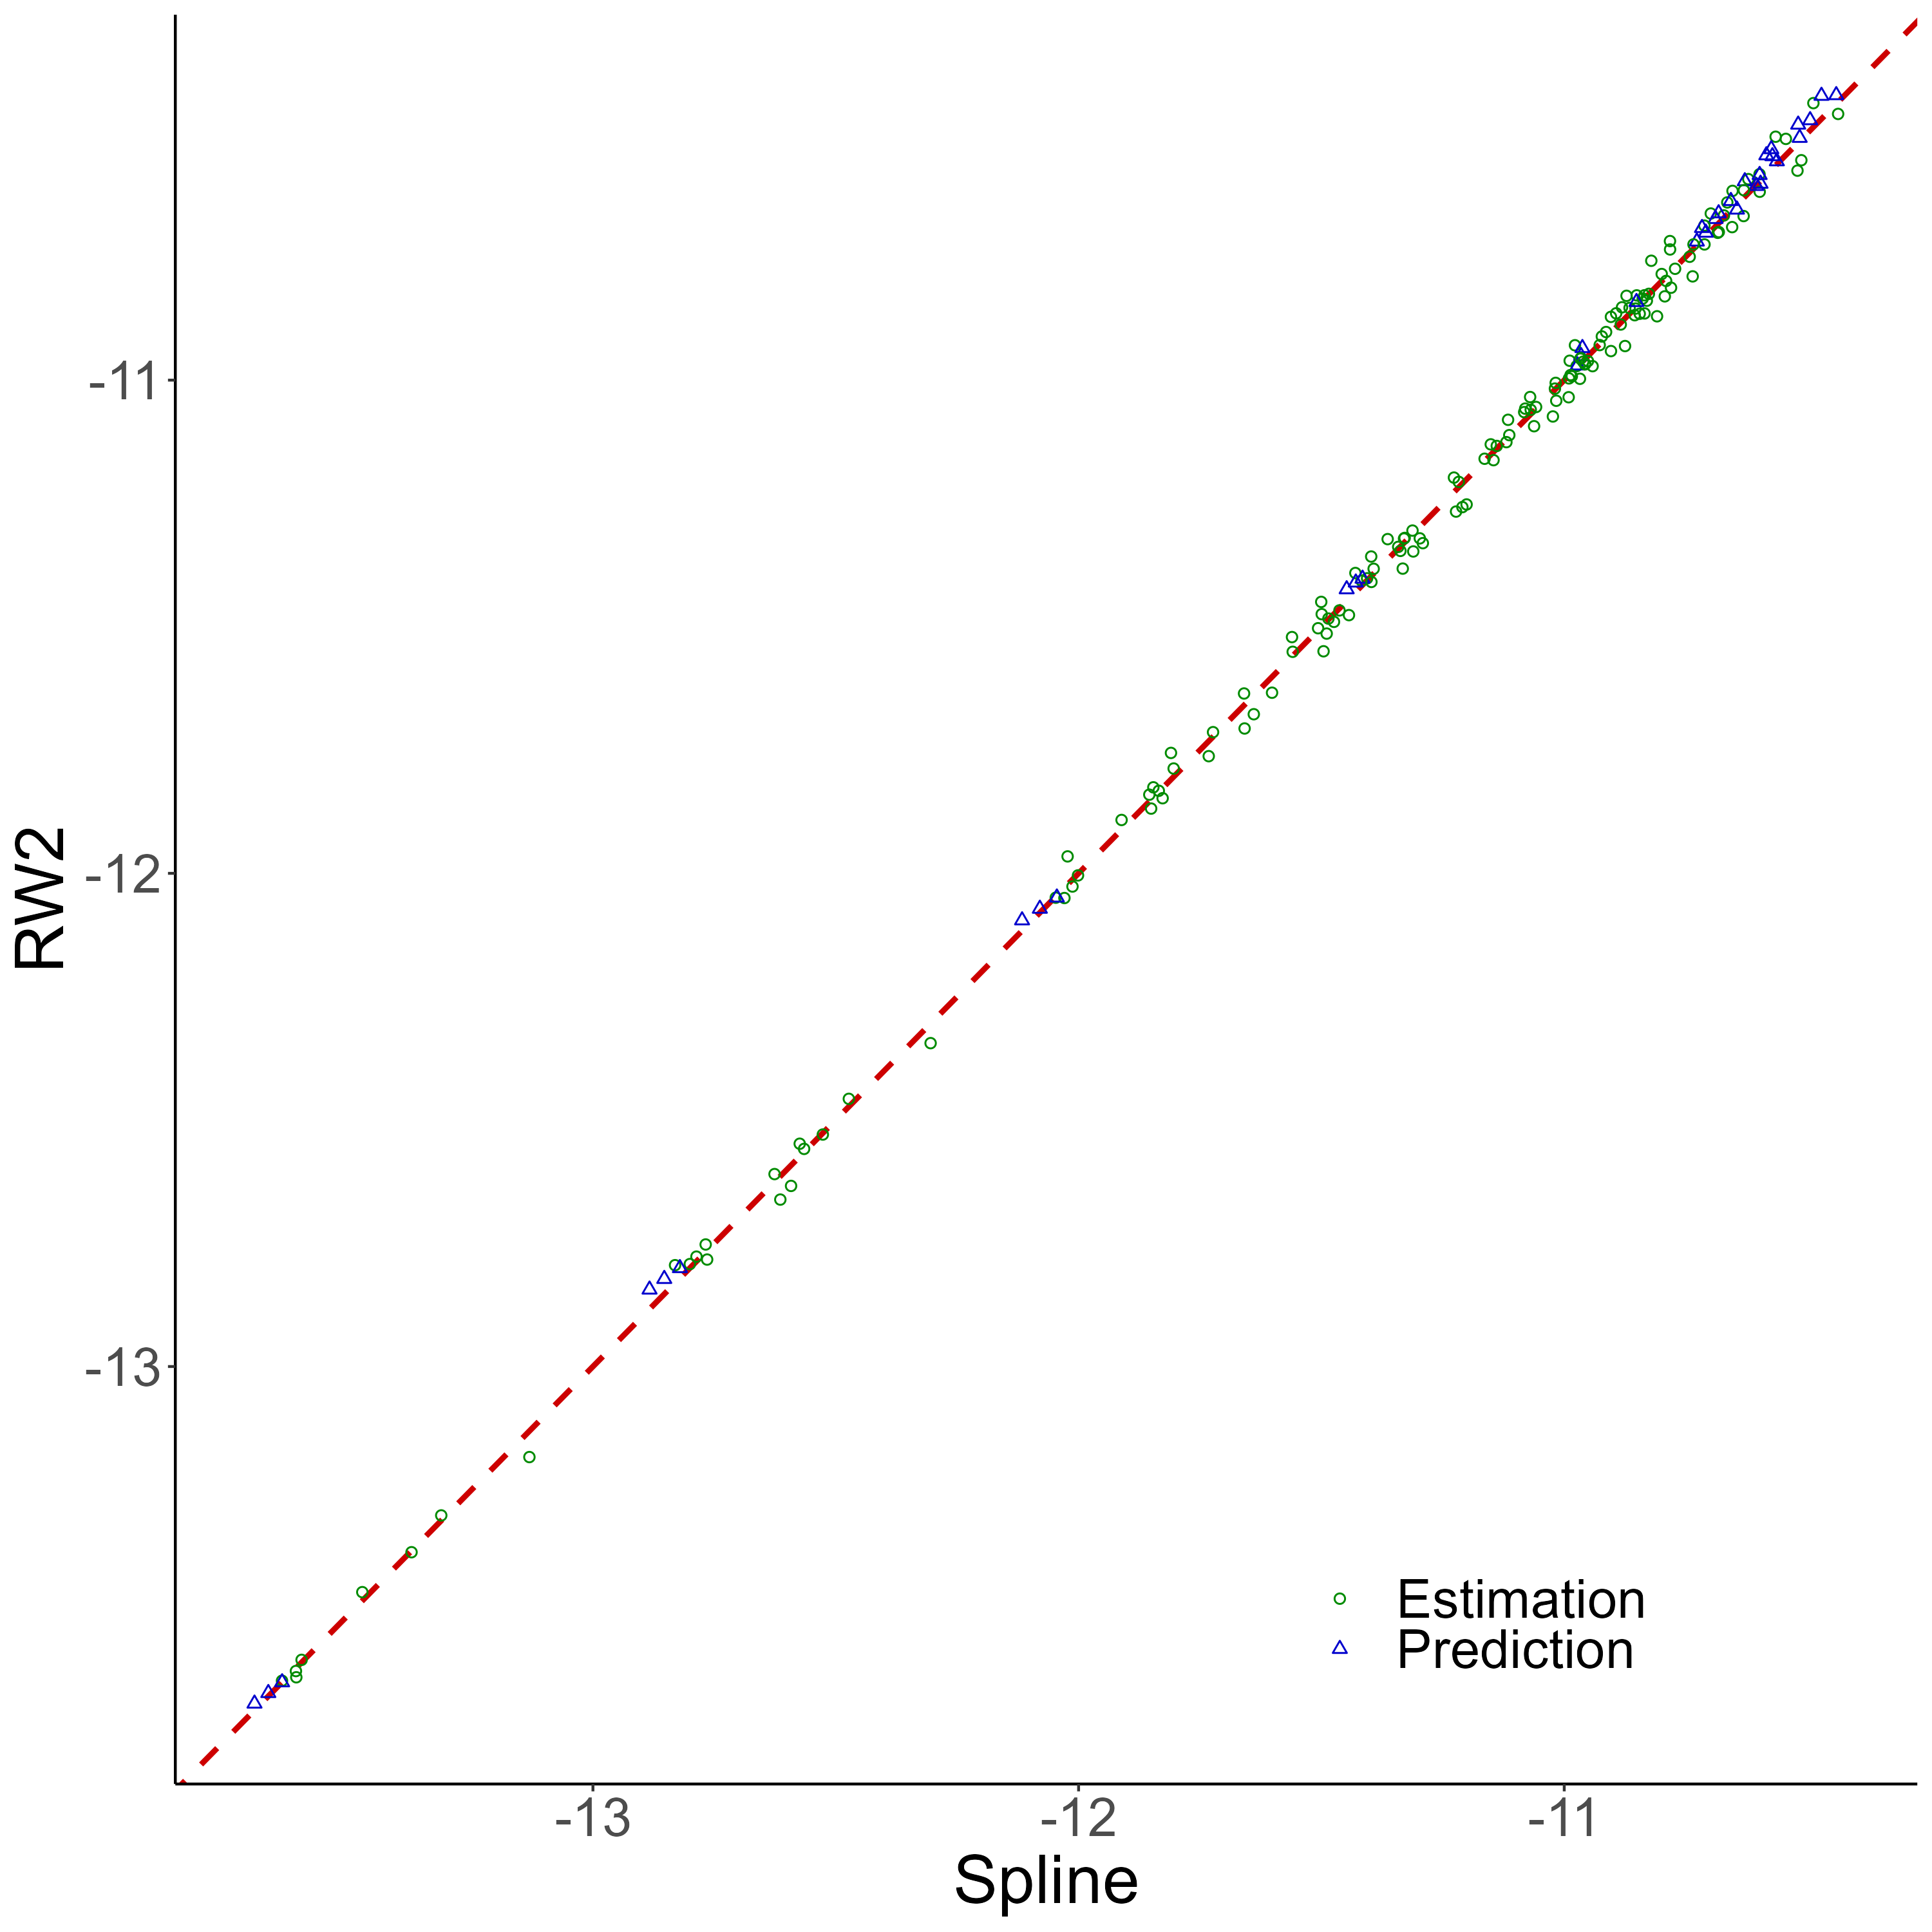}
        \caption{Alcohol related deaths}
        \label{Fig: alcoholPredicted_splineVsRW2}
    \end{subfigure}%
    \begin{subfigure}{.49\textwidth}
        \centering
        \includegraphics[width=\linewidth]{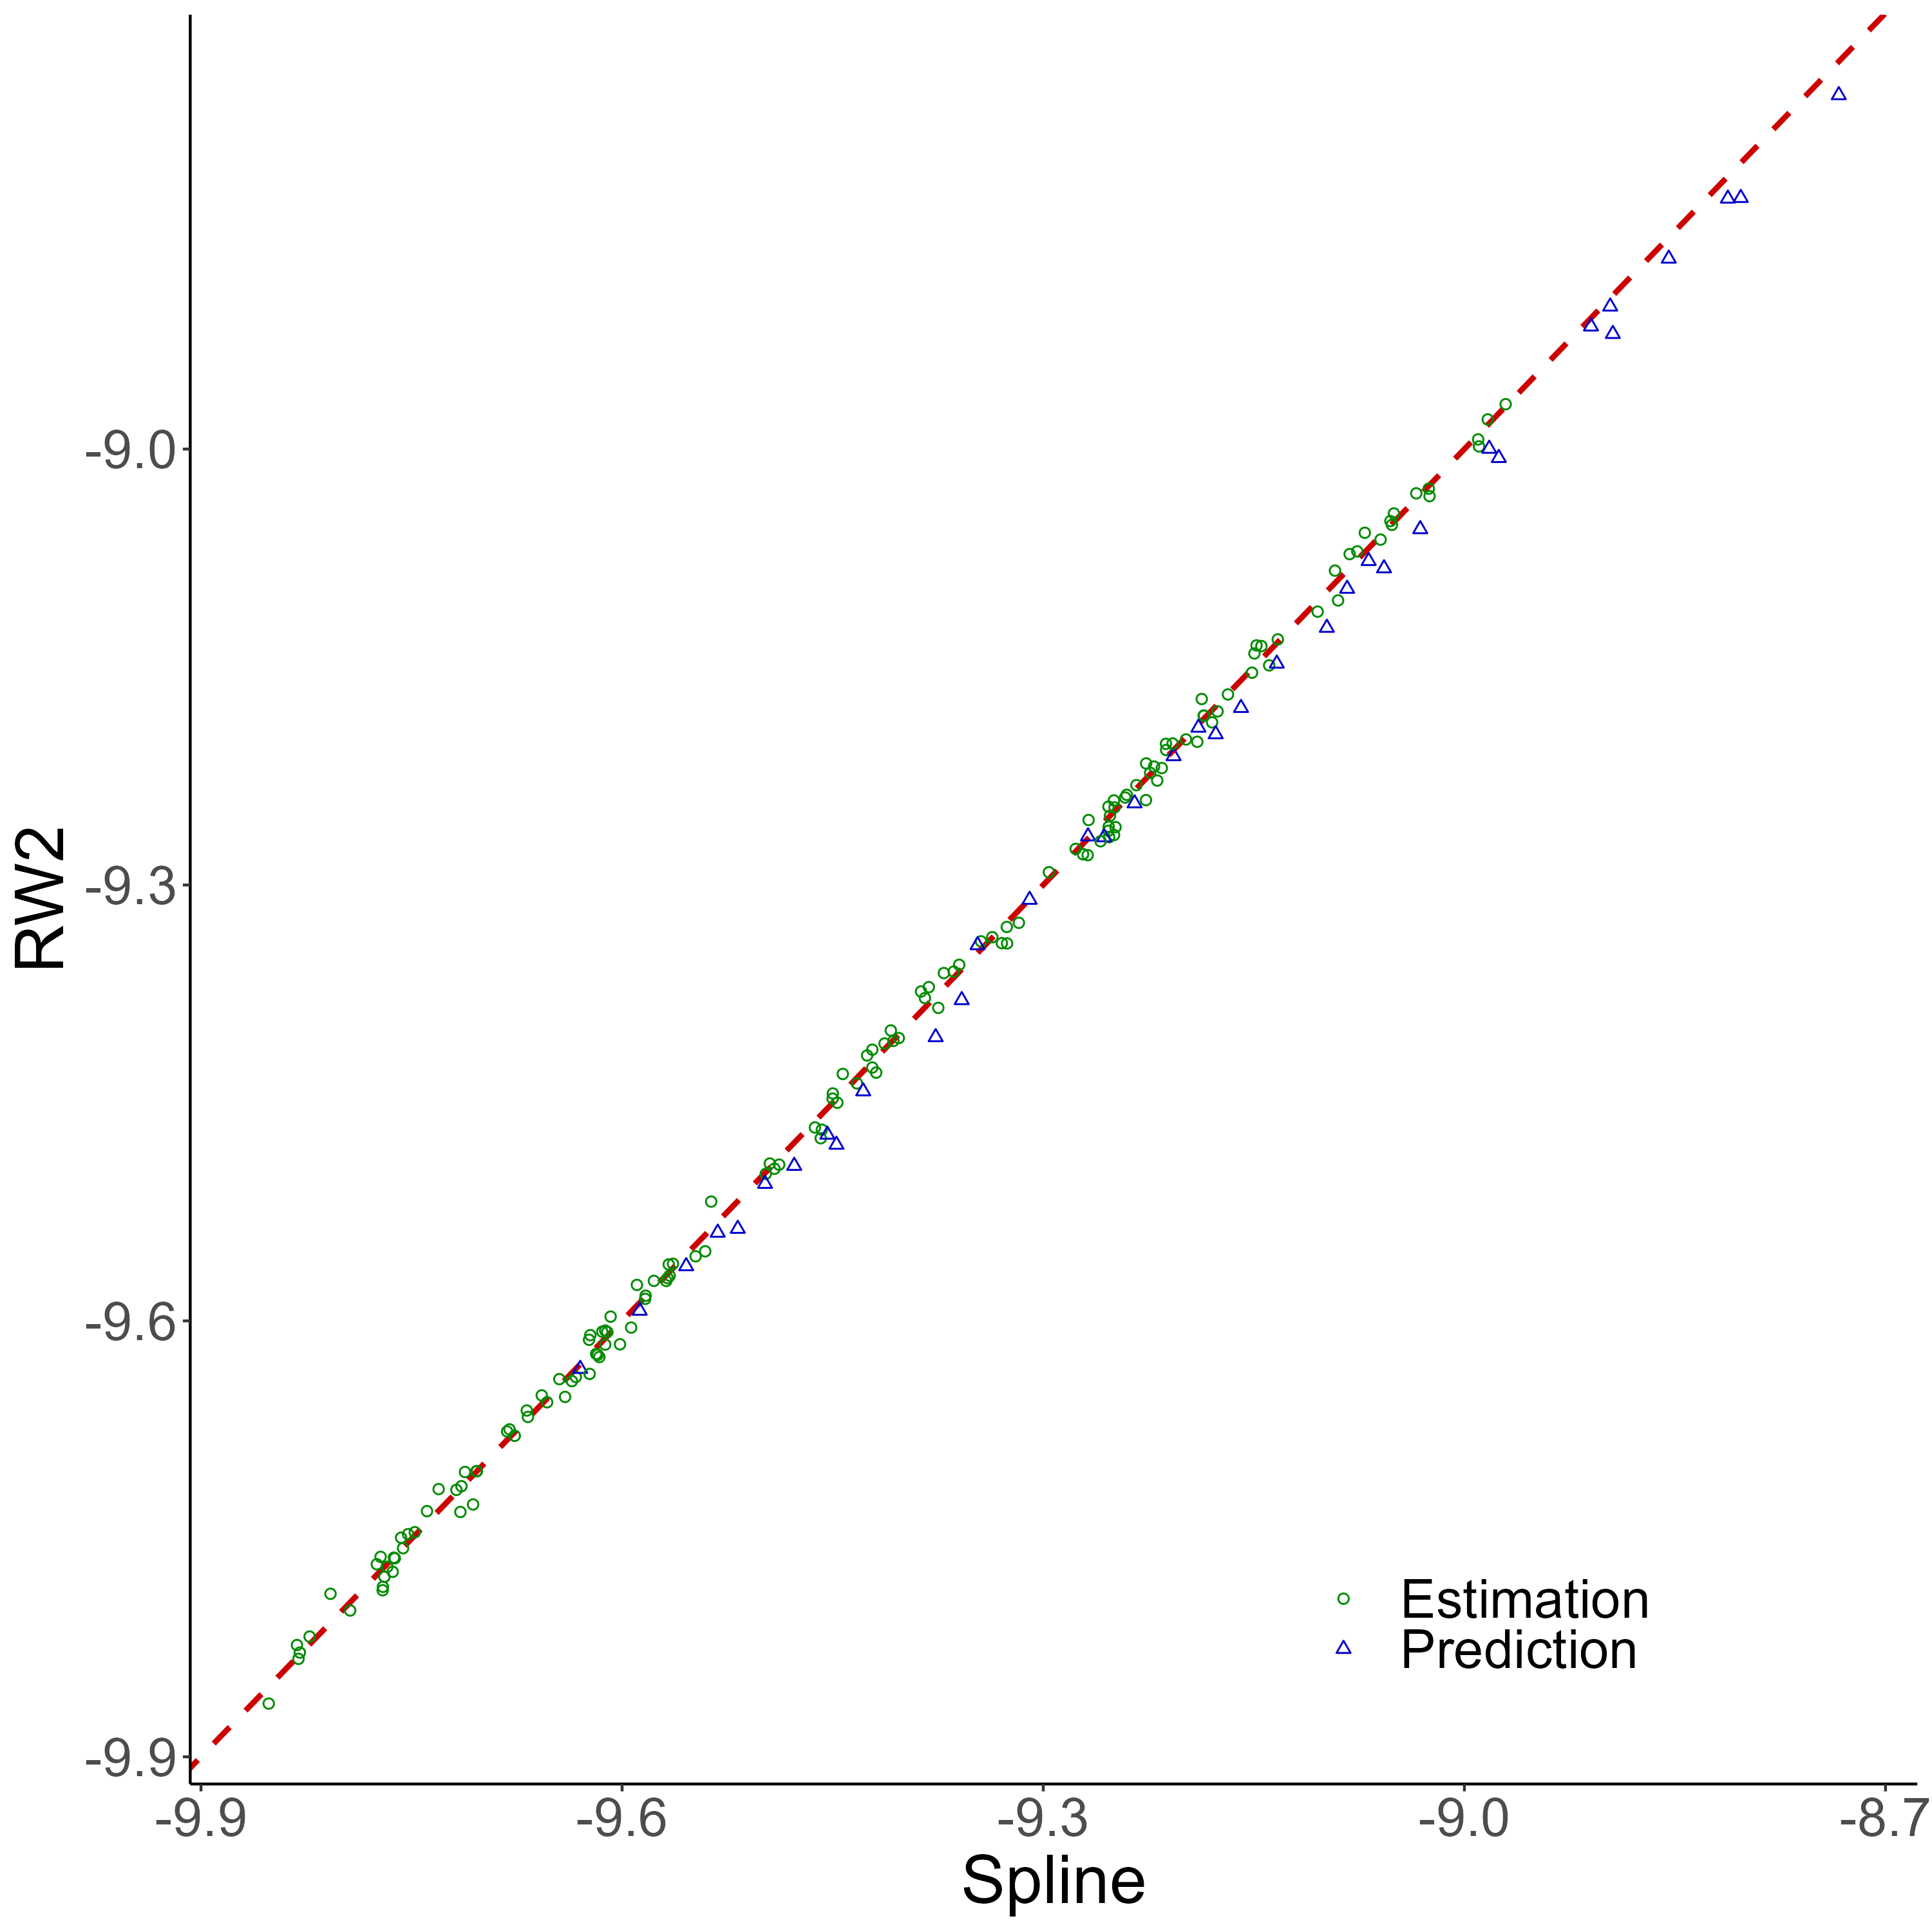}
        \caption{Self harm related deaths}
        \label{Fig: selfHarmPredicted_splineVsRW2}
    \end{subfigure}
    \caption{Comparison of the estimated and in-sample predicted alcohol (a) and self harm (b) related suicide values from the spline and random walk 2 model. In each subfigure, the spline values are along the $x$-axis and the random walk 2 values are on the $y$-axis. The red dotted line is the $y=x$ axis. The green circles and blue triangles represent the estimated and predicted values, respectively.}
    \label{Fig: Predicted_splineVsRW2}
\end{figure}
